# Supplementary material for: Towards Accurate and Consistent Evaluation: A Dataset for Distantly-Supervised Relation Extraction
Source: arXiv:2010.16275 source file (2020-10-30)
Supplement: Supplementary file 1 [file appendix.tex]

% \documentclass[11pt,a4paper]{article}

% \usepackage{times}
% \usepackage{latexsym}
% \usepackage{listings}
% \usepackage{booktabs}
% \usepackage{url}
% \usepackage{graphicx}
% \usepackage{appendix}
% \usepackage{multicol}
% \usepackage{caption}
% \usepackage{subcaption}
% \usepackage[ruled, linesnumbered]{algorithm2e}
% \usepackage{amsmath}
% \usepackage{amssymb}
% \usepackage{float}
% \usepackage{multirow}
% \usepackage{multicol}
% \usepackage{adjustbox}
% \graphicspath{{./misc/}}

% \begin{document}

% \title{Supplemental Material}
% \date{}
% \maketitle

\section{Appendix}

\subsection{Data Details}
There are many data files in the original NYT10, organised in a protocol buffer format. We use the protobuf \footnote{https://developers.google.com/protocol-buffers} tools to extract entities from \texttt{\small filtered-freebase-
simple-topic-dump-3cols.tsv}, and all the entities' \texttt{guid}, \texttt{word} and \texttt{type} attributes come from this file.
All the relations are extracted from files listed as below:
\begin{itemize}
    \item \texttt{\small kb\_manual/trainPositive.pb}
    \item \texttt{\small kb\_manual/trainNegative.pb}
    \item \texttt{\small heldout\_relations/trainPositive.pb}
    \item \texttt{\small heldout\_relations/trainNegative.pb}
    \item \texttt{\small heldout\_relations/testPositive.pb}
    \item \texttt{\small heldout\_relations/testNegative.pb}
\end{itemize}

Figure \ref{fig:datastats} shows a brief overview of NYT-H, and the distribution of sentence length are almost the same.
About half of the bags have only one instance, especially in the NA set with the ratio of 84.75\%. 
The distance histograms indicate that the relative distance between entity pair in most sentences is within 20, which is a reasonable value to express the semantic relation between entity pairs.

\begin{figure*}[ht]
    \centering
    \begin{subfigure}[t]{0.3\textwidth}
        \centering
        \includegraphics[width=\textwidth]{misc/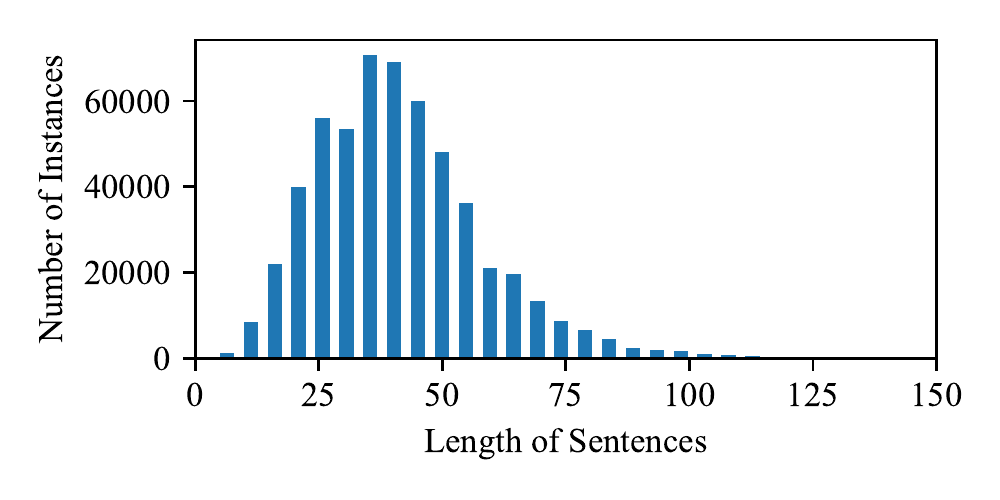}
        \caption{NA Set Distribution of Sentence Length}
        \label{fig:nasentlen}
    \end{subfigure}
    \hfill
    \begin{subfigure}[t]{0.3\textwidth}
        \centering
        \includegraphics[width=\textwidth]{misc/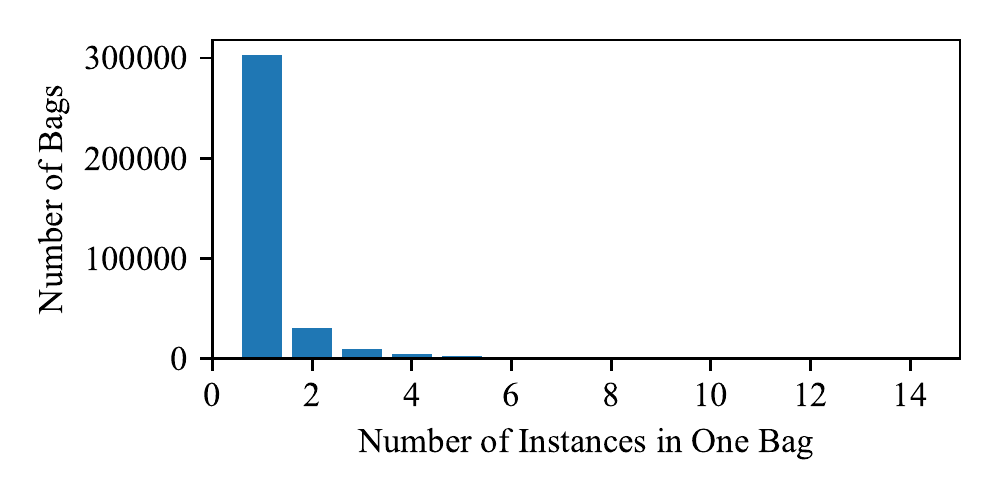}
        \caption{NA Set Number of Instances in Bags}
        \label{fig:nainsinbags}
    \end{subfigure}
    \hfill
    \begin{subfigure}[t]{0.3\textwidth}
        \centering
        \includegraphics[width=\textwidth]{misc/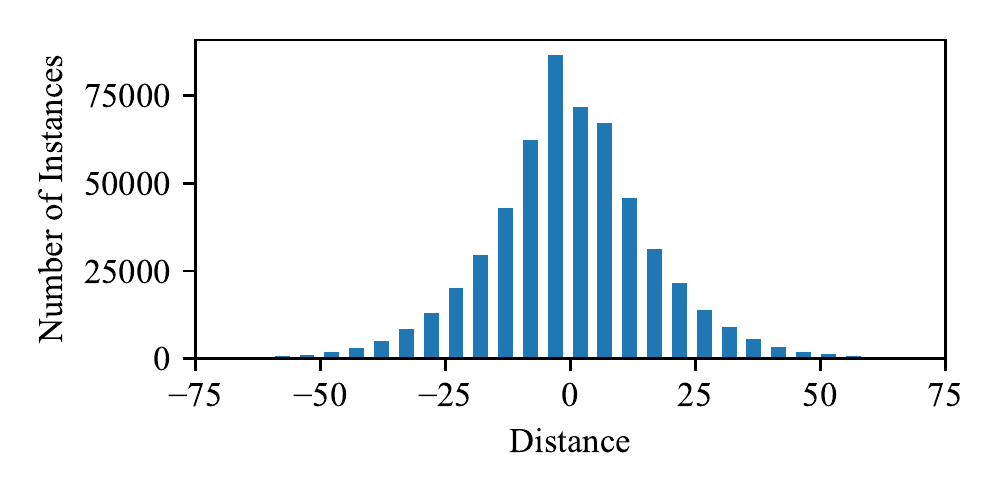}
        \caption{NA Set Distance Between Entities}
        \label{fig:naentdist}
    \end{subfigure}
    \newline
    
    \begin{subfigure}[t]{0.3\textwidth}
        \centering
        \includegraphics[width=\textwidth]{misc/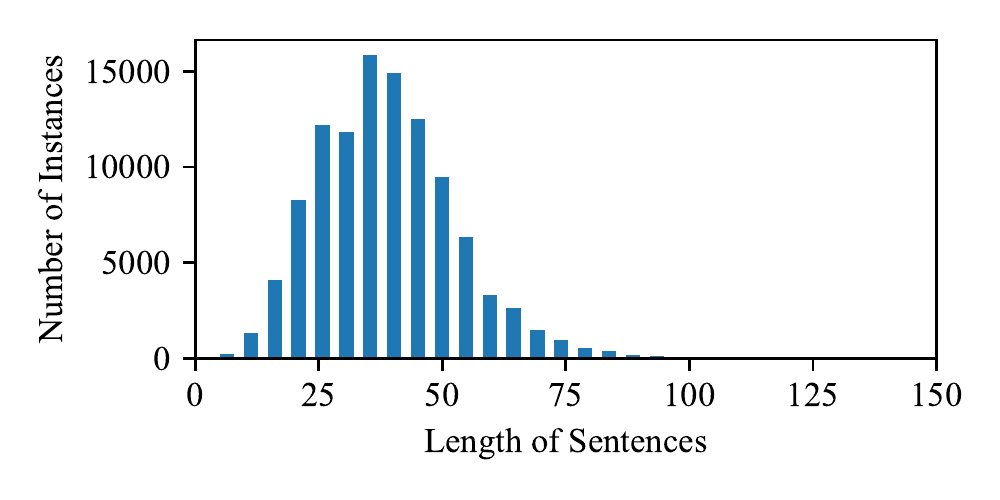}
        \caption{Train Set Distribution of Sentence Length}
        \label{fig:trainsentlen}
    \end{subfigure}
    \hfill
    \begin{subfigure}[t]{0.3\textwidth}
        \centering
        \includegraphics[width=\textwidth]{misc/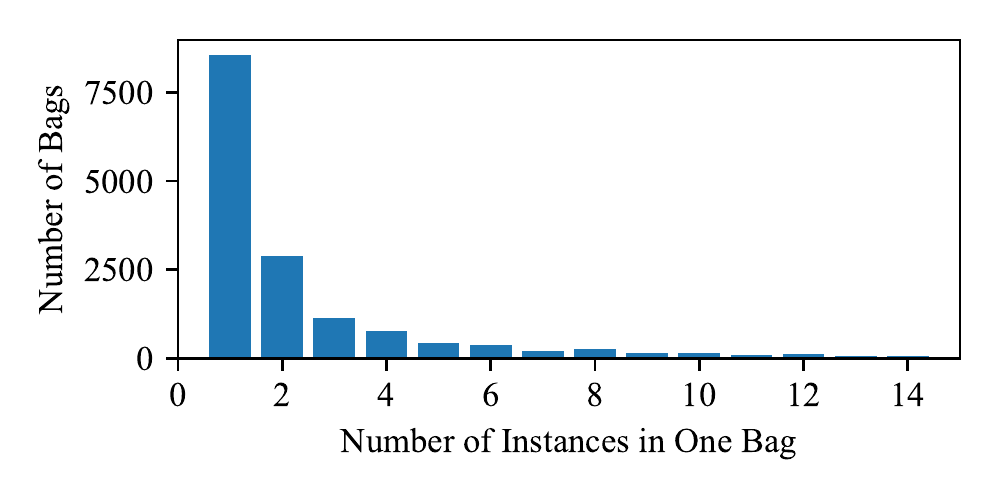}
        \caption{Train Set Number of Instances in Bags}
        \label{fig:traininsinbags}
    \end{subfigure}
    \hfill
    \begin{subfigure}[t]{0.3\textwidth}
        \centering
        \includegraphics[width=\textwidth]{misc/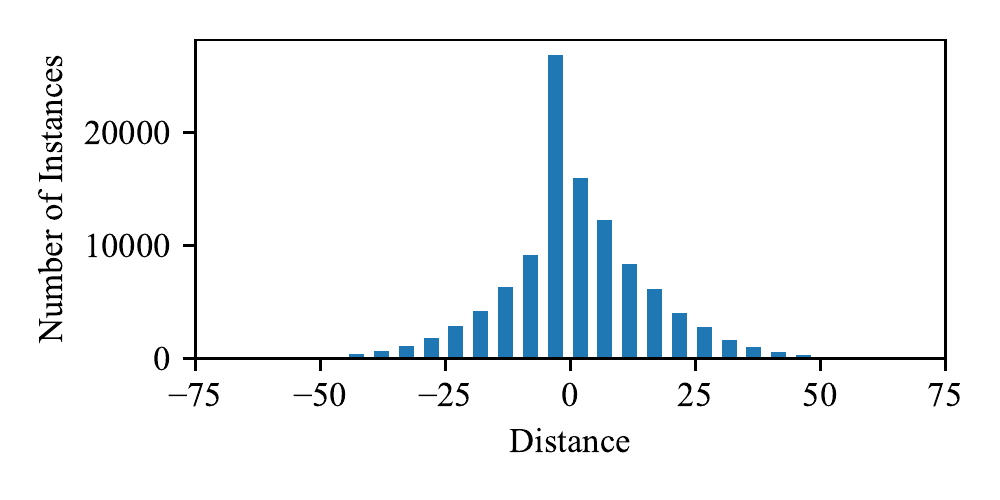}
        \caption{Train Set Distance Between Entities}
        \label{fig:trainentdist}
    \end{subfigure}
    \newline
    
    \begin{subfigure}[t]{0.3\textwidth}
        \centering
        \includegraphics[width=\textwidth]{misc/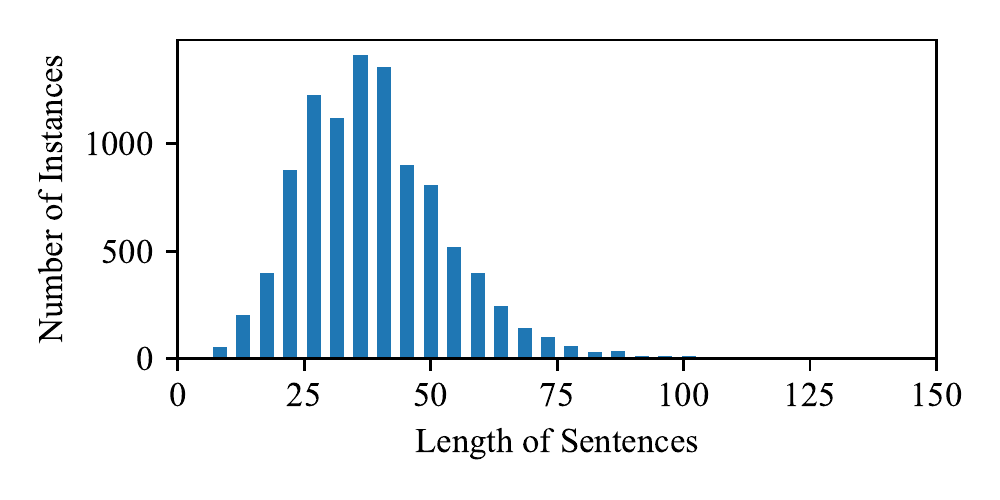}
        \caption{Test Set Distribution of Sentence Length}
        \label{fig:testsentlen}
    \end{subfigure}
    \hfill
    \begin{subfigure}[t]{0.3\textwidth}
        \centering
        \includegraphics[width=\textwidth]{misc/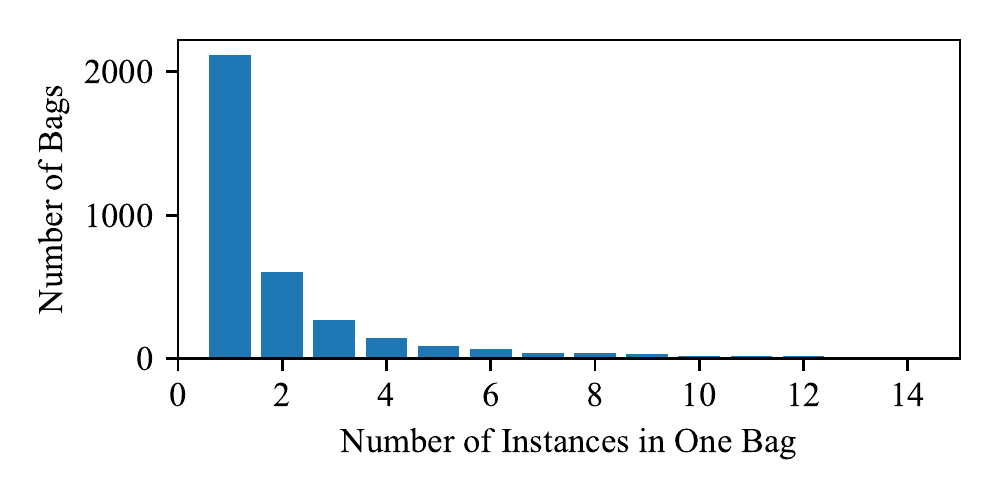}
        \caption{Test Set Number of Instances in Bags}
        \label{fig:testinsinbags}
    \end{subfigure}
    \hfill
    \begin{subfigure}[t]{0.3\textwidth}
        \centering
        \includegraphics[width=\textwidth]{misc/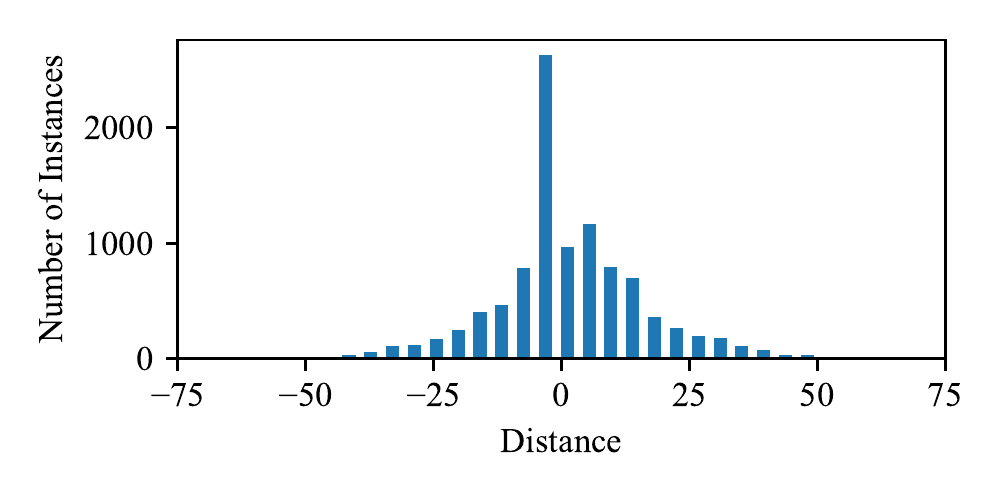}
        \caption{Test Set Distance Between Entities}
        \label{fig:testentdist}
    \end{subfigure}
    
    \caption[Data Statistics]{The lengths of sentences are counted in word level. All the bar plot and the histogram plot are center aligned to the x coordinates. The distance between head entity and tail entity is obtained by subtracting the position of the head entity from the position of the tail entity.}
    \label{fig:datastats}
\end{figure*}

An example of an instance can be found in Figure \ref{fig:ins_example}. And the data details on relations can be found on Table \ref{tab:trainset_count} and Table \ref{tab:testset_count}.

\begin{figure*}
    \centering
    \begin{lstlisting}[breaklines=true,basicstyle=\small\ttfamily,frame=single]
{
    "instance_id": "1",
    "bag_id": "1",
    "relation": "/location/location/contains",
    "bag_label": "yes",
    "head": {
        "guid": "/guid/f0e3",
        "word": "Connecticut",
        "type": "/base/litcentral/topic,/location/administrative_division"
    },
    "tail": {
        "guid": "/guid/b1cc",
        "word": "Farmington",
        "type": "/location/citytown,/location/statistical_region"
    },
    "sentence": "Born in Philadelphia , Pennsylvania on May 1st , 1918 , daughter of the late John and Emma Hallowell , she attended Miss Porters School in Farmington , Connecticut , where she and her husband Theodore later lived for fifty years .",
}
    \end{lstlisting}
    \caption[Instance Example]{The example data is simplified on entity words' \textit{guid} and \textit{type}. If one instance is not annotated, the corresponding bag label will be \textit{unk}.}
    \label{fig:ins_example}
\end{figure*}

\subsection{Parameter Settings}\label{sec:exp_setting}
The detailed parameter settings can be found at Table \ref{tab:parameter_settings}.

\begin{table*}[ht]
    \centering
    \scalebox{0.8}{
        \begin{tabular}{c|c|c}
             \toprule
             & Parameters & Settings  \\
             \midrule
             \midrule
             \multirow{6}{6em}{General}& Word Embedding & GloVe-50d\footnote{\url{https://nlp.stanford.edu/projects/glove/}} \\
             &Position Feature Dim & 5 \\
             &Epoch & 50 \\
             &Batch Size & 64 \\
             &Dropout Rate & 0.5 \\
             &Learning Rate & $1\times10^{-3}$ (with Adam optimizer) \\
             \midrule
             \multirow{2}{6em}{CNN}&Convolutional Filter Num & 230 \\
             &Convolutional Window & 3 \\
             \midrule
             \multirow{4}{6em}{CR-CNN}&Positive Margin & 2.5 \\
             &Negative Margin & 0.5 \\
             &$\gamma$ & 2.0 \\
             &$\beta$ & $1\times10^{-3}$ \\
             \midrule
             \multirow{5}{6em}{ATT-BLSTM}&Embedding Dropout & 0.3 \\
             &LSTM Dropout & 0.3 \\
             &Linear Dropout & 0.5 \\
             &LSTM Hidden Size & 100 \\
             &L2 Decay & $1\times10^{-5}$\\
             \bottomrule
        \end{tabular}
    }
    \caption{Experiments Parameter Settings}
    \label{tab:parameter_settings}
\end{table*}

% train set sent & bags

\begin{table*}[h]
    \centering
    \begin{tabular}{l|c|c}
        \toprule
        Relation & Instances Number & Bags Number \\
        \midrule
        \midrule
        /location/location/contains  &   51059 &  7291 \\
        /people/person/nationality      &8575&    2270 \\
        /location/country/capital       &7340&    81 \\
        /people/person/place\_lived      &7205&    1883 \\
        /location/country/administrative\_divisions      &6301&    180 \\
        /location/administrative\_division/country       &6279&    351 \\
        /location/neighborhood/neighborhood\_of  &5629&    462 \\
        /business/person/company        &5602&    1354 \\
        /people/person/place\_of\_birth   &3084&    982 \\
        /people/deceased\_person/place\_of\_death  &1914&    595 \\
        /business/company/founders      &808&     175 \\
        /location/us\_state/capital      &684&     4 \\
        /people/ethnicity/geographic\_distribution       &531&     26 \\
        /people/person/children & 479     &205 \\
        /business/company/place\_founded &464&     162 \\
        /business/company/major\_shareholders    &291&     25 \\
        /sports/sports\_team\_location/teams      &208&     71 \\
        /sports/sports\_team/location    &204&     71 \\
        /people/ethnicity/people        &150&     54 \\
        /people/person/ethnicity        &145&     54 \\
        /people/person/religion &141&     74 \\
        \midrule
        SUM & 107093 & 16370\\
        \bottomrule
    \end{tabular}
    \caption{Information on Relations in Train Set}
    \label{tab:trainset_count}
\end{table*}

% test set sent & bags
\begin{table*}[h]
    \centering
    \begin{tabular}{l|c|c}
        \toprule
        Relation & Instances Number & Bags Number \\
        \midrule
        \midrule
        /location/location/contains     &4475&    1558 \\
        /people/person/nationality      &1128&    523 \\
        /people/person/place\_lived      &861&     401 \\
        /business/person/company        &591&     277 \\
        /location/country/capital       &570&     30 \\
        /location/administrative\_division/country       &503&     98 \\
        /location/country/administrative\_divisions      &481&     63 \\
        /people/person/place\_of\_birth   &383&     219 \\
        /people/deceased\_person/place\_of\_death  &193&     107 \\
        /location/neighborhood/neighborhood\_of  &176&     83 \\
        /business/company/founders      &149&     51 \\
        /people/ethnicity/geographic\_distribution       &137&     5 \\
        /business/company/place\_founded &57&      33 \\
        /people/person/children &57&      42 \\
        /location/us\_state/capital      &50&      7 \\
        /business/company/major\_shareholders    &47&      9 \\
        /sports/sports\_team/location    &28&      13 \\
        /people/person/religion &28&      10 \\
        /people/person/ethnicity        &22&      7 \\
        /sports/sports\_team\_location/teams      &14&      7 \\
        /people/ethnicity/people        &5&       5 \\
        \midrule
        SUM & 9955 & 3548\\
        \bottomrule
    \end{tabular}
    \caption{Information on Relations in Test Set}
    \label{tab:testset_count}
\end{table*}
